# Supplementary material for: Shape Representation by Zippable Ribbons
Source: arXiv:1711.02450 source file (2017-11-07)
Supplement: Supplementary file 1 [file 07-Appendix.tex]

% !TEX root =  00-Zipper.tex

\section*{Appendix}
